# Supplementary material for: Adaptive Assessment of Visualization Literacy
Source: arXiv:2308.14147 source file (2023-08-27)
Supplement: Supplementary file 1 [file appendix.tex]

\section{Appendix}
% \begin{figure}[h]
%   \centering
%   \includegraphics[width=\columnwidth]{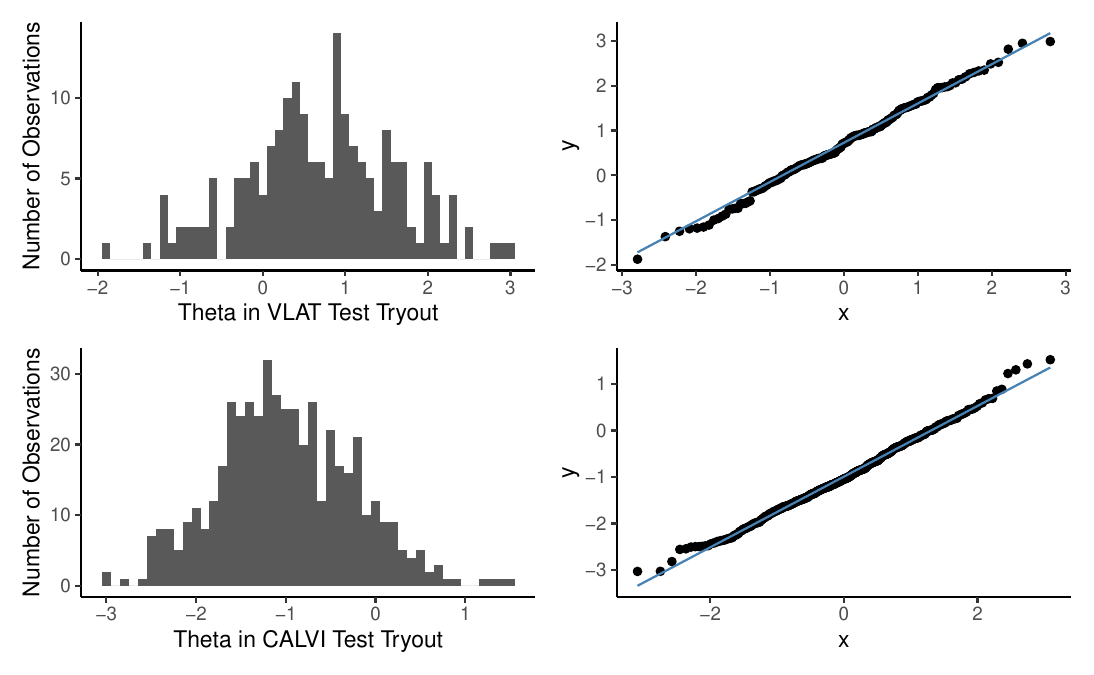}
%   \caption{The distributions of $\theta$ in VLAT and CALVI test tryout data and their Normal quantile-quantile plot. \charles{Is this necessary? If so, how should we present this?}}
% \label{fig:normalityoftheta}
% \end{figure}

\begin{table*}[t]
\centering
    \begin{tabular}{|p{3.2cm}|| p{4.5cm}||p{8.2cm}|}
    \hline
    \textbf{VLAT Chart Types}& 
    \textbf{VLAT Task}&
    \textbf{CALVI Misleader} \\
    \hline
    Area Chart & Determine Range &Cherry Picking \\
    Bar Chart & Identify the Hierarchical Structure   & Concealed Uncertainty \\
    Bubble Chart &Find Anomalies & Inappropriate Aggregation \\
    Choropleth Map &Find Clusters & Manipulation of Scales - Inappropriate Order \\
    Histogram & Find Correlations/Trends & Manipulation of Scales -
Inappropriate Scale Range \\
    Line Chart & Find Extremum & Manipulation of Scales -
Inappropriate Use of
Scale Functions   \\
    Pie Chart & Make Comparisons & Manipulation of Scales -
Unconventional
Scale Directions \\
    Scatterplot & Retrieve Value & Misleading Annotations \\
    Stacked Area Chart &  & Missing Data \\
    Stacked Bar Chart &  & Missing Normalization \\
    Treemap &  & Overplotting \\
    100\% Stacked Bar Chart &  &  \\
    \hline
    \end{tabular}
    \caption{VLAT Chart Types, \textsc{vlat} Tasks, and \textsc{calvi} Misleaders
    \fy{the aesthetics of this table need to be improved .. right now, I feel it is not acceptable...at least remove the two left and right most bars, bold the top and bottom lines} \matt{+1, but also: semantically, this is not a single table, as rows are meaningless. The design should reflect the meaning}\fy{BTW, I don't think you need this table. the content isn't used very much in the text. and I think you can basically write into the two paragraphs/subsections about \textsc{vlat} and \textsc{calvi} I mentioned} \charles{we can make 3 separate tables and align them horizontally? TODO}
    }
    \label{tab:1}
\end{table*}
